# Supplementary material for: Understanding two-dimensional tractor magnets: theory and realizations
Source: arXiv:2405.06402 source file (2024-05-10)
Supplement: Supplementary file 1 [file Supplementary.pdf]

# Supplementary Material to "Understanding two-dimensional tractor magnets: theory and realizations"

Michael P. Adams[a]

*Department of Physics and Materials Science, University of Luxembourg, 162A avenue de la Faiencerie, L-1511 Luxembourg, Grand Duchy of Luxembourg*

(Dated: 1 May 2024)

[a]Electronic address: michael.adams@uni.lu

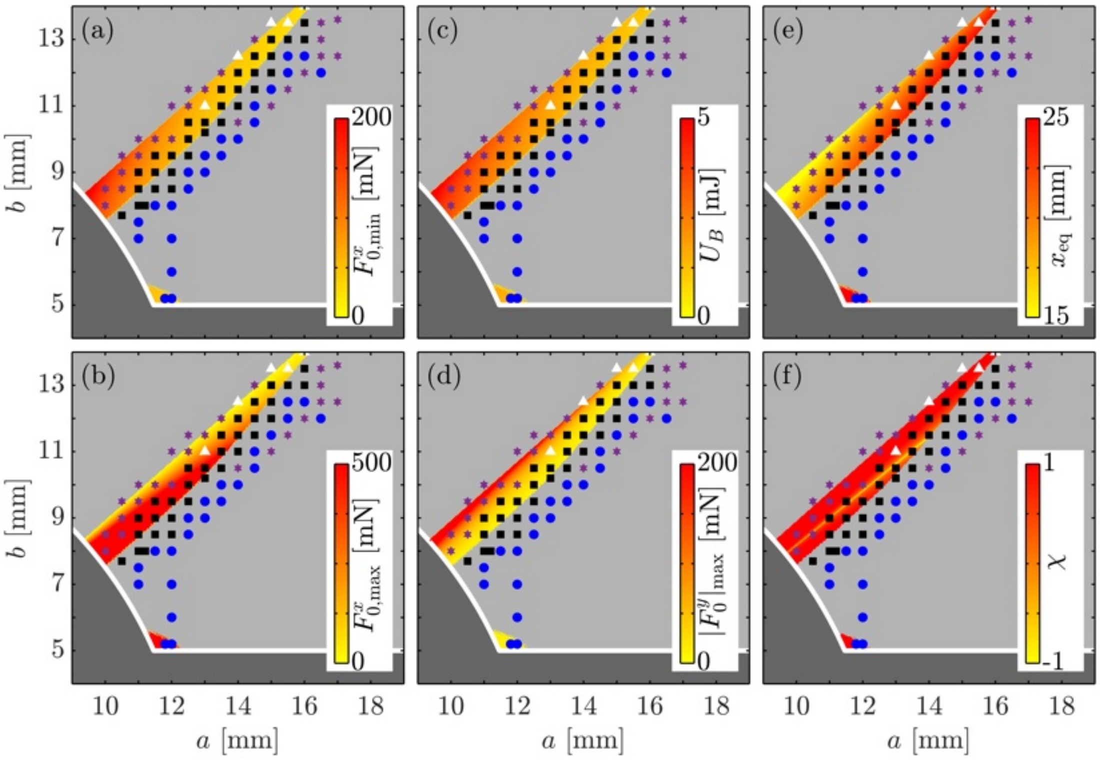


FIG. 1. Same as Fig. 4 in the main article, but with MPEX0 method.

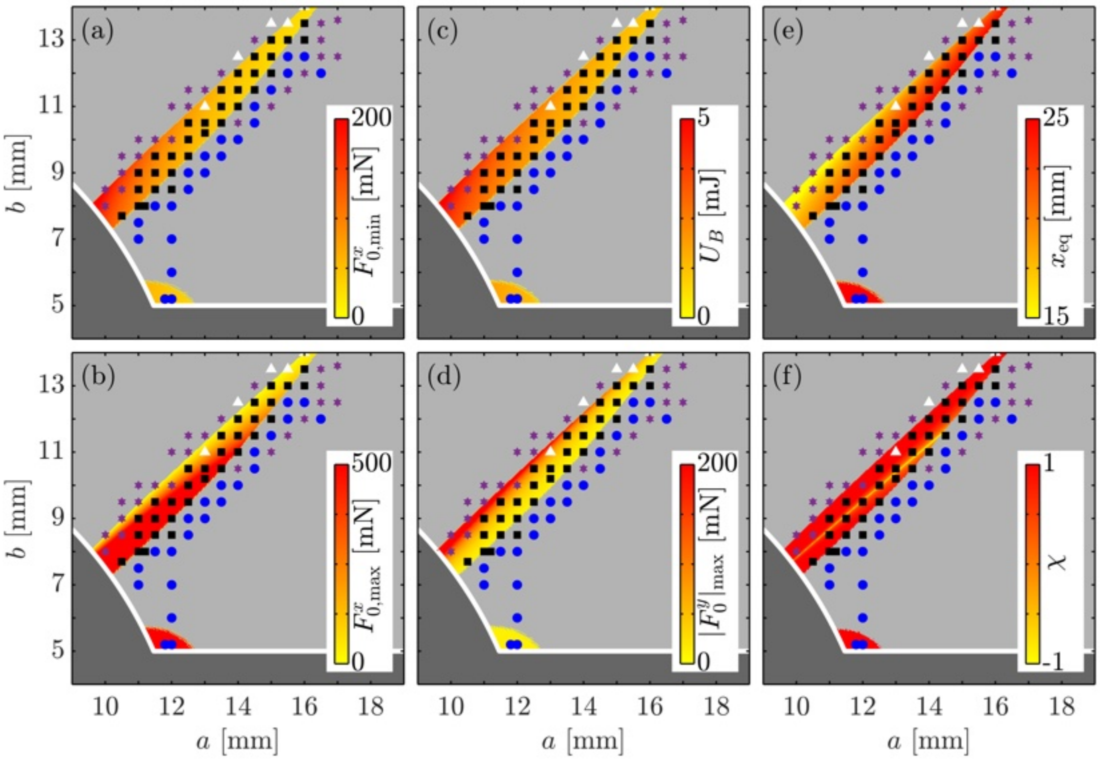


FIG. 2. Same as Fig. 4 in the main article, but with MPEX2 method.

TABLE I. Parameters of the minimal tractor magnet configuration: example I

| Magnet Properties | Remanence $B^{\mathrm{r}} = \mu_0 M^{\mathrm{r}}$ [mT] | Radius $r$ [mm] | Height $h$ [mm] | Mass [g] |
|---|---|---|---|---|
| Ferrite Magnet | 390 | 5 | 5 | 1.96 |
| NdFeB Magnet | 1300 | 7.5 | 5 | 6.63 |

| Magnet List | Position $x_i$ [mm] | Position $y_i$ [mm] | Polarity $p_i$ | Type |
|---|---|---|---|---|
| Magnet $i = 0$ | $x$ | $y$ | $-1$ | NdFeB |
| Magnet $i = 1$ | $-14$ | 0 | $+1$ | NdFeB |
| Magnet $i = 2$ | 0 | 12 | $-1$ | Ferrite |
| Magnet $i = 3$ | 0 | $-12$ | $-1$ | Ferrite |

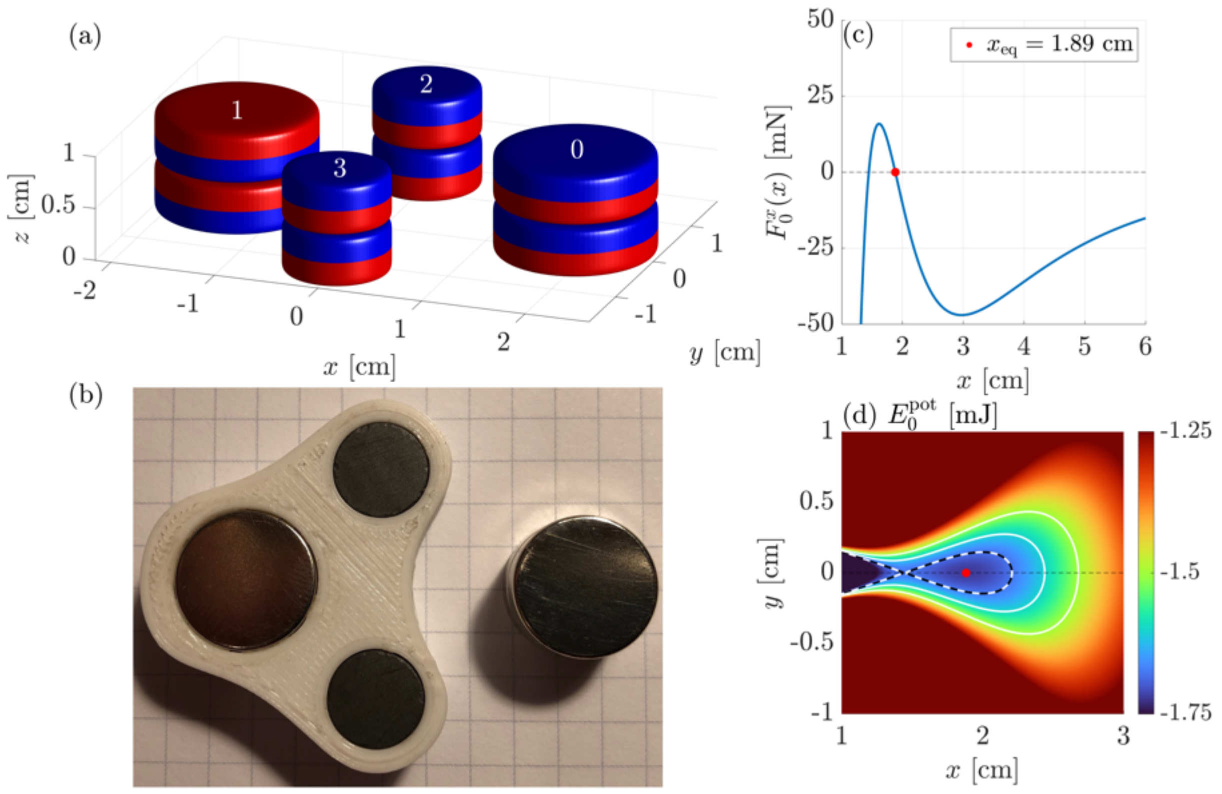


FIG. 3. Realization example I for the minimal tractor magnet configuration. Panel (a) shows a sketch of the magnet configuration with the attractor ($i = 1$), the two repulsors ($i = 2, 3$) and the target ($i = 0$). Panel (b) depicts the corresponding realization. Panel (c) shows the force function component $F_0^x$, and Panel (d) the two-dimensional energy land scape. The red dot in the panels (c) and (d) indicate the stable equilibrium point $x_{\mathrm{eq}}$.

TABLE II. Parameters of the minimal tractor magnet configuration: example II

| Magnet Properties | Remanence $B^r = \mu_0 M^r$ [mT] | Radius $r$ [mm] | Height $h$ [mm] | Mass [g] |
|---|---|---|---|---|
| Ferrite Magnet | 390 | 5 | 5 | 1.96 |
| NdFeB Magnet | 1300 | 7.5 | 5 | 6.63 |
| **Magnet List** | **Position $x_i$ [mm]** | **Position $y_i$ [mm]** | **Polarity $p_i$** | **Type** |
| Magnet $i = 0$ | $x$ | $y$ | $-1$ | NdFeB |
| Magnet $i = 1$ | $-11.2$ | 0 | $+1$ | NdFeB |
| Magnet $i = 2$ | 0 | 8 | $-1$ | Ferrite |
| Magnet $i = 3$ | 0 | $-8$ | $-1$ | Ferrite |

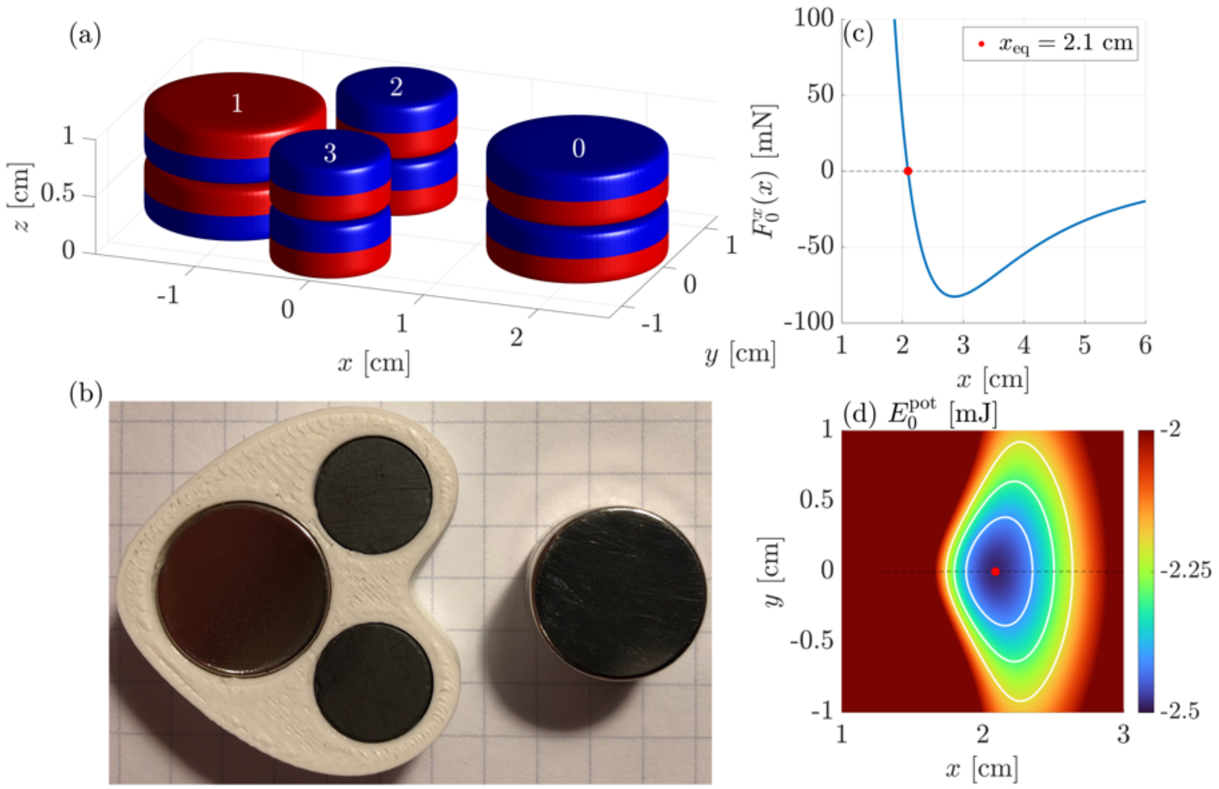


FIG. 4. Same as Fig. 3 for the minimal tractor magnet configuration example II

TABLE III. Parameters of the minimal tractor magnet configuration: example III

| Magnet Properties | Remanence $B^{\mathrm{r}} = \mu_0 M^{\mathrm{r}}$ [mT] | Radius $r$ [mm] | Height $h$ [mm] | Mass [g] |
|---|---|---|---|---|
| Ferrite Magnet | 390 | 5 | 5 | 1.96 |
| NdFeB Magnet | 1300 | 7.5 | 5 | 6.63 |
| **Magnet List** | **Position $x_i$ [mm]** | **Position $y_i$ [mm]** | **Polarity $p_i$** | **Type** |
| Magnet $i = 0$ | $x$ | $y$ | $-1$ | NdFeB |
| Magnet $i = 1$ | $-10.5$ | 0 | $+1$ | NdFeB |
| Magnet $i = 2$ | 0 | 7.7 | $-1$ | Ferrite |
| Magnet $i = 3$ | 0 | $-7.7$ | $-1$ | Ferrite |

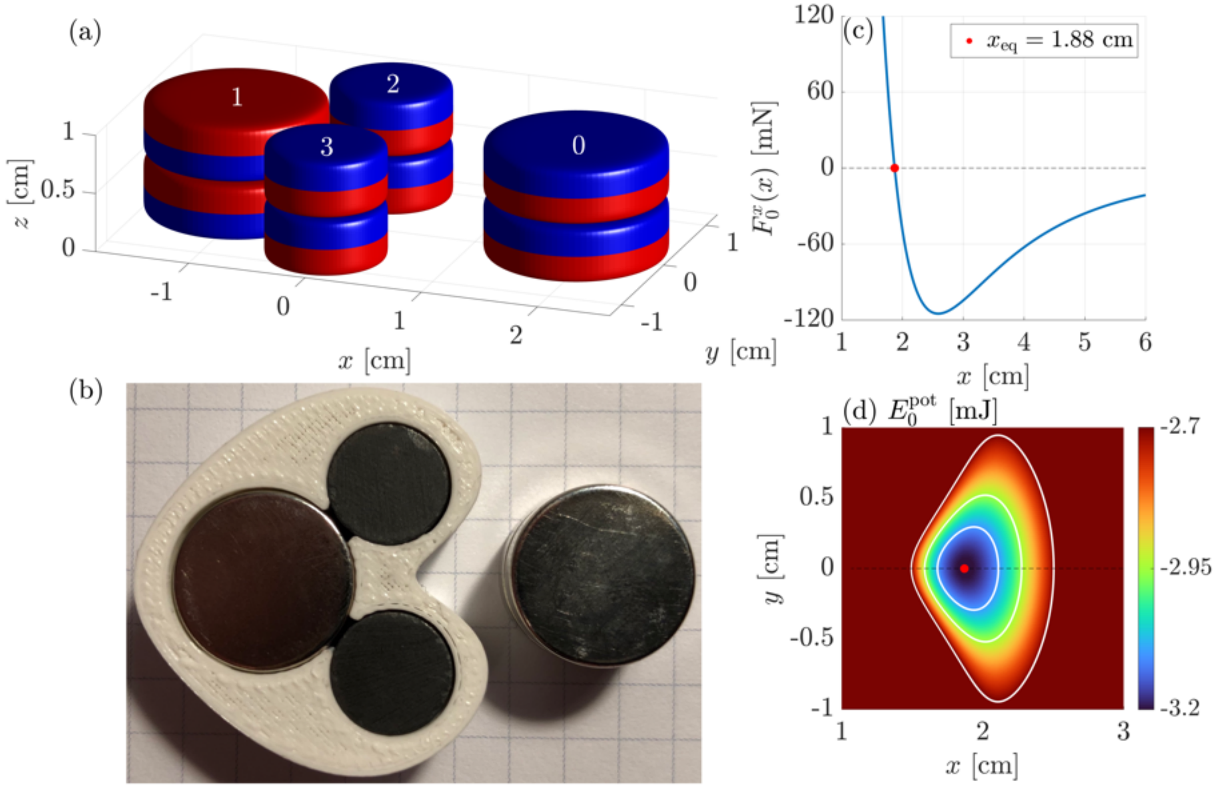


FIG. 5. Same as Fig. 3 for minimal tractor magnet configuration example III

TABLE IV. Parameters of the advanced tractor magnet configuration: example I

| Magnet Properties | Remanence $B^{\mathrm{r}} = \mu_0 M^{\mathrm{r}}$ [mT] | Radius $r$ [mm] | Height $h$ [mm] | Mass [g] |
|---|---|---|---|---|
| Ferrite Magnet | 390 | 5 | 5 | 1.96 |
| NdFeB Magnet | 1300 | 7.5 | 5 | 6.63 |
| **Magnet List** | **Position $x_i$ [mm]** | **Position $y_i$ [mm]** | **Polarity $p_i$** | **Type** |
| Magnet $i = 0$ | $x$ | $y$ | $-1$ | NdFeB |
| Magnet $i = 1$ | $-1.4142$ | $-25.8238$ | $+1$ | NdFeB |
| Magnet $i = 2$ | 0 | $-7.439$ | $-1$ | Ferrite |
| Magnet $i = 3$ | 16.9706 | $-24.4096$ | $-1$ | Ferrite |
| Magnet $i = 4$ | $-1.4142$ | 25.8238 | $+1$ | NdFeB |
| Magnet $i = 5$ | 16.9706 | 24.4096 | $-1$ | Ferrite |
| Magnet $i = 6$ | 0 | 7.439 | $-1$ | Ferrite |

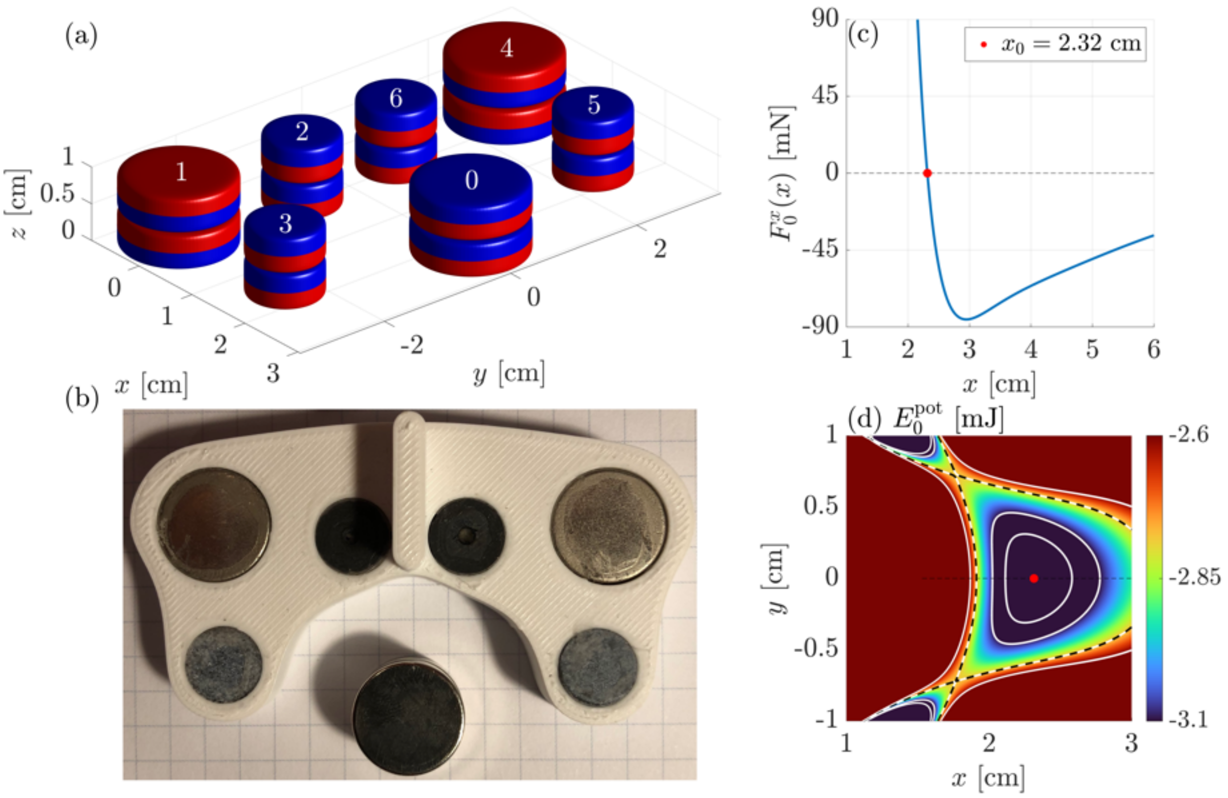


FIG. 6. Same as Fig. 3 for the advanced tractor magnet configuration example I

TABLE V. Parameters of the advanced tractor magnet configuration: example II

| Magnet Properties | Remanence $B^r = \mu_0 M^r$ [mT] | Radius $r$ [mm] | Height $h$ [mm] | Mass [g] |
|---|---|---|---|---|
| Ferrite Magnet | 390 | 5 | 5 | 1.96 |
| NdFeB Magnet | 1300 | 7.5 | 5 | 6.63 |
| **Magnet List** | **Position $x_i$ [mm]** | **Position $y_i$ [mm]** | **Polarity $p_i$** | **Type** |
| Magnet $i = 0$ | $x$ | $y$ | $-1$ | NdFeB |
| Magnet $i = 1$ | $-1.9799$ | $-18.2693$ | $+1$ | NdFeB |
| Magnet $i = 2$ | 0 | $-5.4000$ | $-1$ | Ferrite |
| Magnet $i = 3$ | 10.8894 | $-16.2894$ | $-1$ | Ferrite |
| Magnet $i = 4$ | $-1.9799$ | 18.2693 | $+1$ | NdFeB |
| Magnet $i = 5$ | 10.8894 | 16.2894 | $-1$ | Ferrite |
| Magnet $i = 6$ | 0 | 5.4000 | $-1$ | Ferrite |

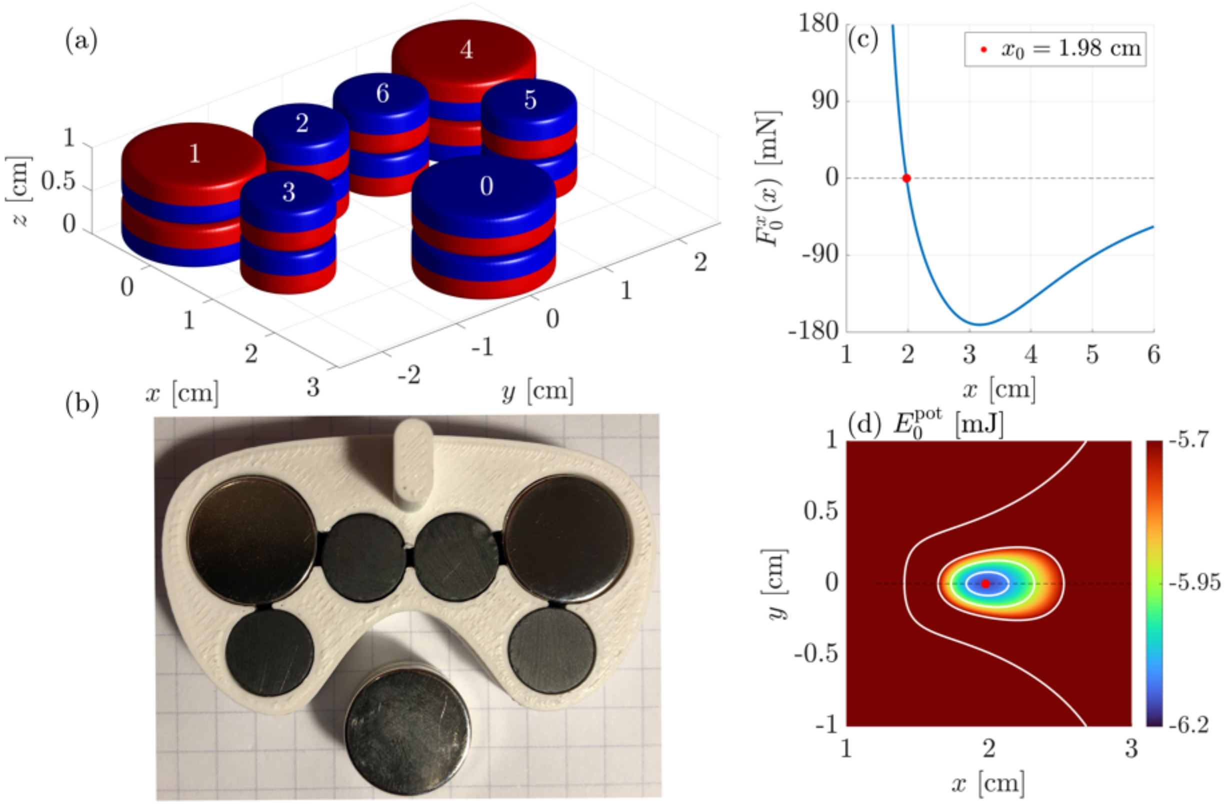


FIG. 7. Same as Fig. 3 for the advanced tractor magnet configuration example II
